# Supplementary material for: Long-lasting Molecular Orientation Induced by a Single Terahertz Pulse
Source: arXiv:2003.01482 ancillary file (2020-03-08)
Supplement: Supplementary file 1 [file sup_inf.pdf]

# Supplementary Information: Long-lasting Orientation Induced by a Single Terahertz Pulse

Long Xu, Ilia Tutunnikov, Erez Gershnabel, Yehiam Prior, and Ilya Sh. Averbukh
*AMOS and Department of Chemical and Biological Physics,*
*The Weizmann Institute of Science, Rehovot 7610001, Israel*

In Note 1, we present the details of our quantum simulation. In Note 2, the molecular properties of the two molecules, methyl chloride and propylene oxide, used in our simulations, are given. In Note 3, the centrifugal distortion effect is discussed. In Note 4, the general solution of motion of free symmetric top is presented. Finally, Note 5 presents the model system of a gas of symmetric top molecules thermalized in a constant dc field which is then abruptly switched off.

## SUPPLEMENTARY NOTE 1: QUANTUM SIMULATION

Hamiltonian describing molecular rotation driven by external time-dependent field interacting with the molecular dipole moment is given by [1]

$$H(t) = H_R + H_{\text{int}}(t), \tag{1}$$

where $H_R$ is the rotational kinetic energy Hamiltonian and $H_{\text{int}}(t) = -\boldsymbol{\mu}\cdot\mathbf{E}(t)$ is the molecule-field interaction. Here $\boldsymbol{\mu}$ is the molecular dipole moment and $\mathbf{E}(t)$ is the external electric field. For the field amplitudes used here, contribution of higher order interaction terms is negligible. For the quantum mechanical treatment, it is convenient to express the Hamiltonian in the basis of free symmetric-top wave functions $|JKM\rangle$ [2]. Here $J$ is the total angular momentum, while $K$ and $M$ denote its projections on the molecule-fixed axis and the laboratory-fixed $Z$ axis, respectively. Matrix elements of the kinetic energy operator of asymmetric-top are given by [2]

$$\langle JKM|H_R|JKM\rangle = \frac{B+C}{2}\left[J(J+1) - K^2\right] + AK^2, \tag{2}$$

$$\langle JKM|H_R|JK\pm 2M\rangle = \frac{B-C}{4} f(J, K\pm 1), \tag{3}$$

where

$$f(J,K) = \sqrt{(J^2-K^2)[(J+1)^2-K^2]}, \tag{4}$$

and the rotational constants are defined by $A = \hbar^2/(2I_a), B = \hbar^2/(2I_b), C = \hbar^2/(2I_c)$ with $A > B > C$.

To simplify the evaluation of matrix element of the Hamiltonian, it is beneficial to express the Hamiltonian in terms of Wigner D-functions. For this, we choose to work in a spherical basis, where the transformation between the laboratory- and molecule-fixed frames reads [2]

$$T_p^{(k)} = \sum_q D^{k\;*}_{pq}(R) T_q^{(k)}. \tag{5}$$

Here, $D^{k\;*}_{pq}(R)$ is the complex conjugate of the Wigner D-matrix and $R$ denotes the set of the three Euler angles, $(\theta,\phi,\chi)$. $T_p^{(k)}$ and $T_q^{(k)}$ represent the spherical irreducible tensors of rank $k$ in the laboratory- and molecule-fixed frames, respectively. The components of $T_p^{(1)}$ are given by $T_{\pm1}^{(1)} = \mp(T_X \pm iT_Y)/\sqrt{2}$ and $T_0^{(1)} = T_Z$. Therefore, the matrix elements of $H_{\text{int}}(t)$ can be rewritten in terms of 3-j symbols as follows

$$\begin{aligned}\langle JKM|H_{\text{int}}(t)|J'K'M'\rangle &= -\sum_{p=-1}^{+1}(-1)^p\langle JKM|\mu_p^{(1)}E_{-p}^{(1)}(t)|J'K'M'\rangle \\ &= -\sum_{p,q=-1}^{+1}(-1)^p\mu_q^{(1)}E_{-p}^{(1)}(t)\langle JKM|D^{1\;*}_{pq}(R)|J'K'M'\rangle,\end{aligned} \tag{6}$$

where the components of dipole moment spherical tensor are defined by $\mu_{\pm1}^{(1)} = \mp(\mu_b \pm i\mu_c)/\sqrt{2}$ and $\mu_0^{(1)} = \mu_a$. The matrix elements on the right hand are given by the relation [2]

$$\langle JKM|D^{1\;*}_{pq}(R)|J'K'M'\rangle = (-1)^{M-K}\sqrt{(2J+1)(2J'+1)}\begin{pmatrix} J & 1 & J' \\ -M & p & M'\end{pmatrix}\begin{pmatrix} J & 1 & J' \\ -K & q & K'\end{pmatrix}. \tag{7}$$

By numerically diagonalization of the rotational Hamiltonian $H_R$, we can determine the asymmetric top eigenfunctions $|J\tau M\rangle = \sum_K c_K^{(J,\tau,M)}|JKM\rangle$. Here, $|J\tau M\rangle$ is composed of symmetric-top wave functions $|JKM\rangle$ with the same

$J$ and $M$ but different $K$, because only the energy levels with different $K$ are coupled in the rotational Hamiltonian [Eq. (3)]. The initial state is chosen as $|\Psi(t=0)\rangle = |J\tau M\rangle$ and the polarization can be expressed as

$$P_i^{(J,\tau,M)}(t) = \langle\Psi(t)|\boldsymbol{\mu}\cdot\mathbf{n}_i|\Psi(t)\rangle = \sum_{p=-1}^{+1}(-1)^p\langle\Psi(t)|\mu_p^{(1)}n_{-p}^{(1)}|\Psi(t)\rangle, \tag{8}$$

where $\mathbf{n}_i$ represents the unit vector $n_X, n_Y, n_Z$ in the laboratory frame. In order to consider the thermal effects, the results for different initial states $|J\tau M\rangle$ are averaged with relative weight given by the Boltzmann distribution

$$P_i(t) = \frac{1}{Z}\sum_{J,\tau,M} P_i^{(J,\tau,M)}(t)\exp\left(-\frac{\varepsilon_{J,\tau,M}}{k_BT}\right), \tag{9}$$

where $Z = \sum_{J,\tau,M}\exp\left(-\varepsilon_{J,\tau,M}/k_BT\right)$ and $\varepsilon_{J,\tau,M}$ is the energy of state $|J\tau M\rangle$.

The calculation for the symmetric-top molecule case is the similar to the asymmetric-top case described above, except that now the eigenstates are $|JKM\rangle$ and the thermal averaging [Eq. (9)] is modified according to

$$P_i(t) = \frac{1}{Z}\sum_{J,K,M} P_i^{(J,K,M)}(t)\epsilon_K\exp\left(-\frac{\varepsilon_{J,K,M}}{k_BT}\right), \tag{10}$$

where $Z = \sum_{J,K,M}\epsilon_K\exp\left(-\varepsilon_{J,K,M}/k_BT\right)$ and the statistical weight $\epsilon_K$ is introduces as a consequence of nuclear spin statistics [3]. For methyl chloride molecule ($CH_3Cl$) considered in this work, the statistical weight is defined by [3]

$$\epsilon_K = \frac{(2I_H+1)^3}{3}\left[1+\frac{2\cos(2\pi K/3)}{(2I_H+1)^2}\right], \tag{11}$$

with $I_H = 1/2$.

## SUPPLEMENTARY NOTE 2: MOLECULAR PROPERTIES

Molecular moments of inertia and the components of molecular dipole moments were computed with the help of GAUSSIAN software package (method: CAM-B3LYP/aug-ccpVTZ) [4]. Supplementary Table 1 summarizes the parameters for $CH_3Cl$ and ($R$)-PPO.

**Supplementary Table 1:** Summary of molecular properties of two molecules (methyl chloride and propylene oxide): eigenvalues of the moment of inertia tensor (atomic units) and components of dipole moment (Debye units) in the body-fixed frame of molecular principal axes.

| Molecules | Moments of inertia | Molecular dipole components |
|---|---|---|
| Methyl chloride | $I_a = 20910$ | $\mu_a = 1.986$ |
| | $I_b = 251506$ | $\mu_b = 0$ |
| | $I_c = 251506$ | $\mu_c = 0$ |
| Propylene oxide | $I_a = 180386$ | $\mu_a = 0.965$ |
| | $I_b = 493185$ | $\mu_b = -1.733$ |
| | $I_c = 553513$ | $\mu_c = 0.489$ |

## SUPPLEMENTARY NOTE 3: EFFECT OF THE CENTRIFUGAL DISTORTION

For a prolate symmetric-top molecule like $CH_3Cl$, the rotational kinetic energy including the contribution of centrifugal distortion is given by [2]

$$\langle JKM|H_{\text{cent}}|JKM\rangle = -D_JJ^2(J+1)^2 - D_{JK}J(J+1)K^2 - D_KK^4, \tag{12}$$

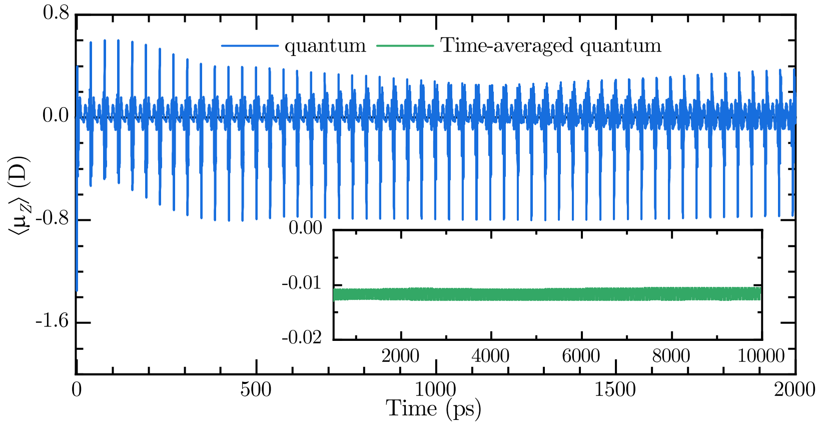


**Supplementary Figure 1:** Ensemble averaged $Z$-projection of the dipole moment, $\langle\mu_Z\rangle$ as a function of time for $CH_3Cl$ molecule. Inset shows the sliding window time average, defined by $\overline{\langle\mu_Z\rangle(t)} = (\Delta t)^{-1}\int_{t-\Delta t/2}^{t+\Delta t/2} \mathrm{d}t'\langle\mu_Z\rangle(t')$ with $\Delta t = 1000$ ps.

where the centrifugal constants of $CH_3Cl$ are $D_J = 18.1$ kHz, $D_{JK} = 197.9$, kHz, and $D_K = 2653.1$ kHz [5].

Supplementary Figure 1 shows the numerical result for molecular orientation dynamics described by the Hamiltonian $H_\mathrm{m} = H_R + H_\mathrm{int} + H_\mathrm{cent}$. The parameters used here are the same as those used in the main text. In particular, the electric field of the THz pulse is modeled as $\mathbf{E}(t) = E_0(1-2\kappa t^2)e^{-\kappa t^2}\mathbf{e}_Z$ [6], where $E_0 = 8.0$ MV/cm and $\kappa = 3.06$ ps$^{-2}$. The initial temperature is set to $T = 5$ K. As shown in Supplementary Figure 1, although the centrifugal distortion affects the amplitude of quantum revivals, the moving window average is essentially not affected by it, resulting in approximately the same persistent value [see Fig. 1(a) in the main text].

## SUPPLEMENTARY NOTE 4: MOTION OF FREE SYMMETRIC TOP

For free symmetric top, prolate for definiteness, the time dependence of a unit vector $\mathbf{a}$, pointing along the symmetry axis of the molecule, is given by a simple vectorial differential equation $\dot{\mathbf{a}} = (\mathbf{L}/I)\times\mathbf{a}$. Here, $\mathbf{L}$ is the angular momentum vector, $I$ is the moment of inertia along the other two axes ($I_a < I_b = I_c \equiv I$). The solution may be found using geometrical arguments and it is given by

$$\mathbf{a}(t) = \mathbf{L}\frac{\mathbf{L}\cdot\mathbf{a}(0)}{L^2} + \left[\mathbf{a}(0) - \mathbf{L}\frac{\mathbf{L}\cdot\mathbf{a}(0)}{L^2}\right]\cos\left(\frac{L}{I}t\right) + \frac{\mathbf{L}}{L}\times\mathbf{a}(0)\sin\left(\frac{L}{I}t\right). \tag{13}$$

The above equation describes precession of the unit vector $\mathbf{a}$ around $\mathbf{L}$ with rate $L/I$, where $L$ is the magnitude of angular momentum.

## SUPPLEMENTARY NOTE 5: PERSISTENT ENSEMBLE AVERAGED ORIENTATION - MODEL SYSTEM

Consider a model system: a gas of prolate symmetric top molecules themalized in a constant dc field of amplitude $E_0$ which is abruptly switched off at some moment (defining $t = 0$). In this case, the distribution of initial conditions is given by the Bolzmann distribution

$$P(L, L_a, \theta) = \frac{1}{\mathcal{Z}}\exp\left\{-\frac{L^2}{2Ik_BT}\left[1 + \frac{L_a^2}{L^2}(w-1)\right] + \frac{\mu E_0}{k_BT}\cos\theta\right\}, \tag{14}$$

where $\mathcal{Z}$ is the partition function, $T$ is temperature, $k_B$ is the Bolzmann constant, $L_a$ is the projection of the angular momentum on the $a$ axis (symmetry axis), $w = I/I_a$, $I_a$ is the moment of inertia along the $a$ axis, $\mu$ is the magnitude of the molecular dipole, and $\theta$ is the angle between molecular dipole ($a$ axis) and the direction of the dc field (laboratory $Z$ axis). The persistent ensemble averaged dipole is given by

$$\frac{\overline{\langle \mu_Z \rangle}}{\mu} = \lim_{\tau\to\infty} \frac{1}{\mathcal{Z}} \int \frac{1}{\tau} \int\limits_0^\tau \mathbf{a}(t)\cdot \mathbf{Z} \exp\left\{-\frac{L^2}{2Ik_BT}\left[1+\frac{L_a^2}{L^2}(w-1)\right] + \epsilon\cos\theta\right\} \mathrm{d}t\mathrm{d}\Lambda, \tag{15}$$

where $\mathbf{Z}$ is the unit vector along laboratory $Z$ axis, $\epsilon \equiv \mu E_0/k_BT$ and $\mathrm{d}\Lambda$ denotes integration over all the parameters, which will be introduced below. Integration over time results in

$$\frac{\overline{\langle \mu_Z \rangle}}{\mu} = \frac{1}{\mathcal{Z}} \int \frac{L_a L_Z}{L^2} \exp\left\{-\frac{L^2}{2Ik_BT}\left[1+\frac{L_z^2}{L^2}(w-1)\right] + \epsilon\cos\theta\right\} \mathrm{d}\Lambda, \tag{16}$$

where we used Eq. (13) to obtain

$$\lim_{\tau\to\infty} \frac{1}{\tau} \int\limits_0^\tau \mathbf{a}(t)\cdot\mathbf{Z}\mathrm{d}t = \mathbf{L}\cdot\mathbf{Z}\frac{\mathbf{L}\cdot\mathbf{a}(0)}{L^2} = \frac{L_a L_Z}{L^2}. \tag{17}$$

Projection of the angular momentum $L_a$ can be expressed in terms of $L_X$, $L_Y$, $L_Z$, and the three Euler angles [2]

$$L_a = L_X \sin\theta\cos\phi + L_Y \sin\theta\sin\phi + L_Z\cos\theta. \tag{18}$$

Denoting $L_Z/L = \cos\theta_1$, we explicitly write the resulting integral

$$\frac{\overline{\langle \mu_Z \rangle}}{\mu} = \frac{1}{\mathcal{Z}} \int \cos^2\theta_1 \cos\theta \exp\left\{-\frac{L^2}{2Ik_BT}\left[1+\cos^2\theta_1(w-1)\right] + \epsilon\cos\theta\right\} L^2 \sin\theta_1 \sin\theta \mathrm{d}\chi\mathrm{d}\phi\mathrm{d}\theta\mathrm{d}\theta_1\mathrm{d}L. \tag{19}$$

Notice that terms proportional to $\cos\phi$ and $\sin\phi$ do not contribute to the ensemble averaged dipole moment, since the dc field doesn't affect the uniform distribution of the angle $\phi$. Change of variables $x = \cos\theta$, $y = \cos\theta_1$ and $l = L/\sqrt{2Ik_BT}$ results in

$$\begin{aligned}\frac{\overline{\langle \mu_Z \rangle}}{\mu} &= \frac{4\pi^2}{\mathcal{Z}}(2Ik_BT)^{3/2} \int\limits_{-1}^{1} x e^{\epsilon x}\mathrm{d}x \int\limits_{-1}^{1}\int\limits_0^\infty y^2 e^{-l^2\left[1+y^2(w-1)\right]} l^2 \mathrm{d}l\mathrm{d}y \\ &= \frac{4\pi^2}{\mathcal{Z}} 2(2Ik_BT)^{3/2} \frac{\epsilon\cosh(\epsilon)-\sinh(\epsilon)}{\epsilon^2} \int\limits_{-1}^{1}\int\limits_0^\infty y^2 e^{-l^2\left[1+y^2(w-1)\right]} l^2 \mathrm{d}l\mathrm{d}y \\ &= \frac{4\pi^2}{\mathcal{Z}}\frac{\sqrt{\pi}}{2}(2Ik_BT)^{3/2}\frac{\epsilon\cosh(\epsilon)-\sinh(\epsilon)}{\epsilon^2}\mathcal{I}_1(w),\end{aligned} \tag{20}$$

where

$$\mathcal{I}_1(w) = \int\limits_{-1}^{1} \frac{y^2\mathrm{d}y}{\left[1+y^2(w-1)\right]^{3/2}}.$$

The partition function $\mathcal{Z}$ is given by

$$\begin{aligned}\mathcal{Z} &= \int \exp\left[-\frac{L^2}{2Ik_BT}\left[1+\frac{L_z^2}{L^2}(w-1)\right] + \epsilon\cos\theta\right]\mathrm{d}\Lambda \\ &= 4\pi^2(2Ik_BT)^{3/2}\int\limits_{-1}^{1} e^{\epsilon x}\mathrm{d}x \int\limits_{-1}^{1}\int\limits_0^\infty e^{-l^2\left[1+y^2(w-1)\right]} l^2\mathrm{d}l\mathrm{d}y \\ &= 4\pi^2\frac{\sqrt{\pi}}{2}(2Ik_BT)^{3/2}\frac{\sinh(\epsilon)}{\epsilon}\mathcal{I}_2(w).\end{aligned} \tag{21}$$

where

$$\mathcal{I}_2(w) = \int\limits_{-1}^{1} \frac{\mathrm{d}y}{\left[1+y^2(w-1)\right]^{3/2}}.$$

Substitution of the partition function yields

$$\overline{\langle\mu_Z\rangle} = \mu\frac{\epsilon\cosh\epsilon - \sinh\epsilon}{\epsilon\sinh\epsilon}\frac{\mathcal{I}_1(w)}{\mathcal{I}_2(w)}. \tag{22}$$

Notice that in presence of dc field at thermal equilibrium, the ratio $\mathcal{I}_1/\mathcal{I}_2 = 1$. When $\epsilon \to 0$, $\overline{\langle\mu_Z\rangle} \to 0$. The factor $\mathcal{I}_1(w)/\mathcal{I}_2(w) \le 1/3$, and for $w = 1$ the ratio is equal $1/3$.


[1] R. V. Krems, *Molecules in Electromagnetic Fields: From Ultracold Physics to Controlled Chemistry* (Wiley, 2018).

[2] Richard N Zare, *Angular momentum: understanding spatial aspects in chemistry and physics* (Wiley, New York, 1988).

[3] Robin S. McDowell, "Rotational partition functions for symmetrictop molecules," J. Chem. Phys. **93**, 2801–2811 (1990).

[4] M. J. Frisch, G. W. Trucks, H. B. Schlegel, G. E. Scuseria, M. A. Robb, J. R. Cheeseman, G. Scalmani, V. Barone, G. A. Petersson, H. Nakatsuji, X. Li, M. Caricato, A. V. Marenich, J. Bloino, B. G. Janesko, R. Gomperts, B. Mennucci, H. P. Hratchian, J. V. Ortiz, A. F. Izmaylov, *et al.*, "Gaussian 16 Revision A. 03, Gaussian Inc. Wallingford CT," (2016).

[5] G. M. Black and M. M. Law, "The general harmonic force field of methyl chloride," J. Mol. Spectrosc. **205**, 280–285 (2001).

[6] L. H. Coudert, "Optimal orientation of an asymmetric top molecule with terahertz pulses," J. Chem. Phys. **146**, 024303 (2017).
